# Supplementary material for: UltraFlux: Data-Model Co-Design for High-quality Native 4K Text-to-Image Generation across Diverse Aspect Ratios
Source: arXiv:2511.18050 source file (2025-11-22)
Supplement: Supplementary file 1 [file supp-1-1-visual_comparison_compressed.pdf]

*A woman with a chic hairstyle wears elegant eyeglasses and multiple pieces of jewelry, including earrings and layered necklaces, against a textured gray background.*

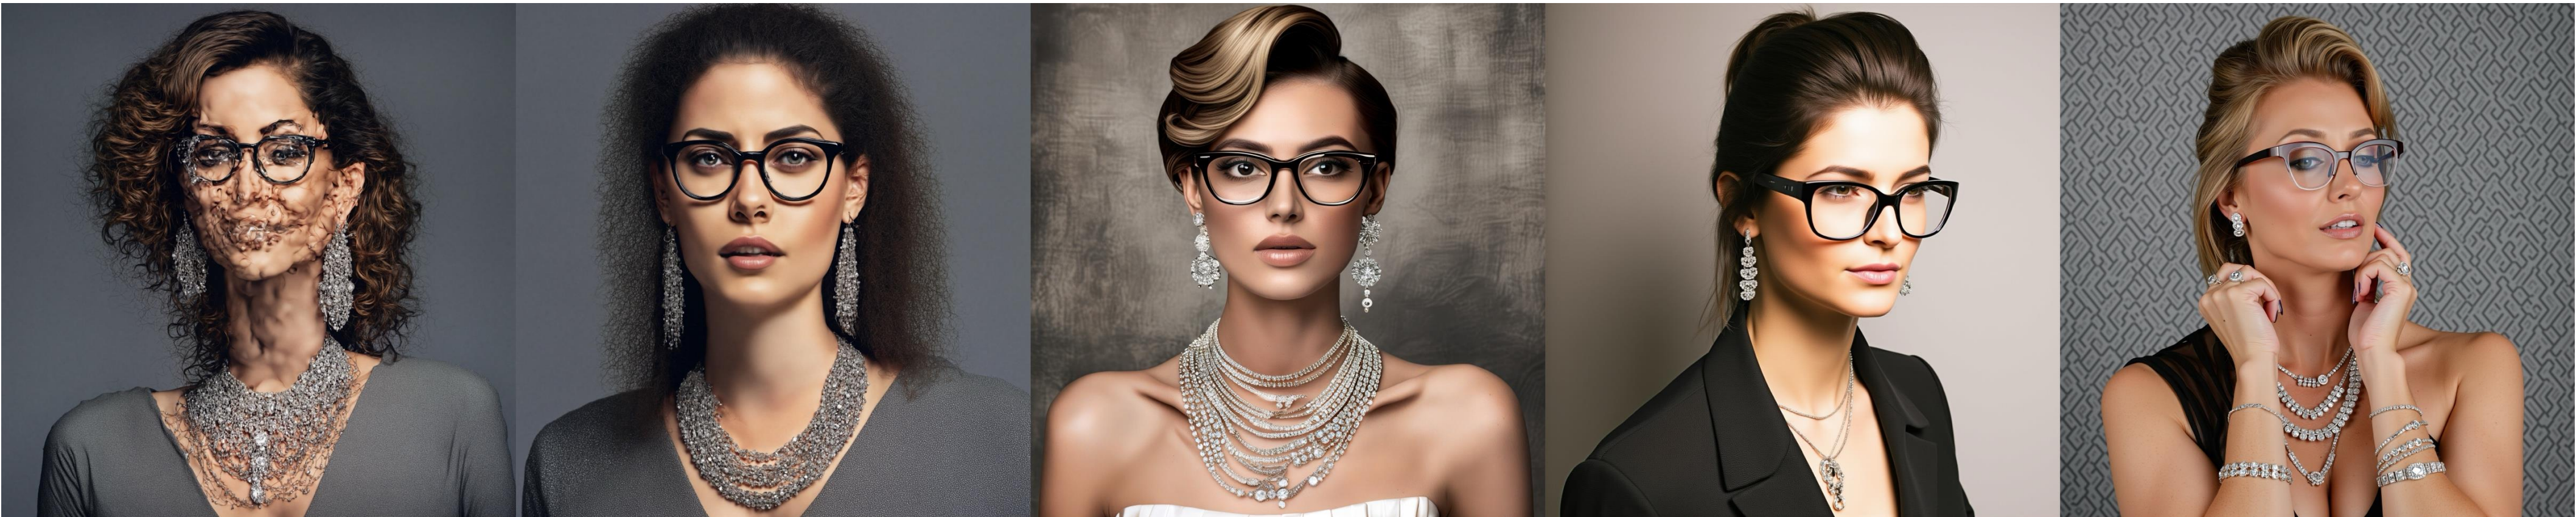

*Blonde model with tousled hair wearing a form-fitting olive green dress, looking intently at the camera with a soft expression.*

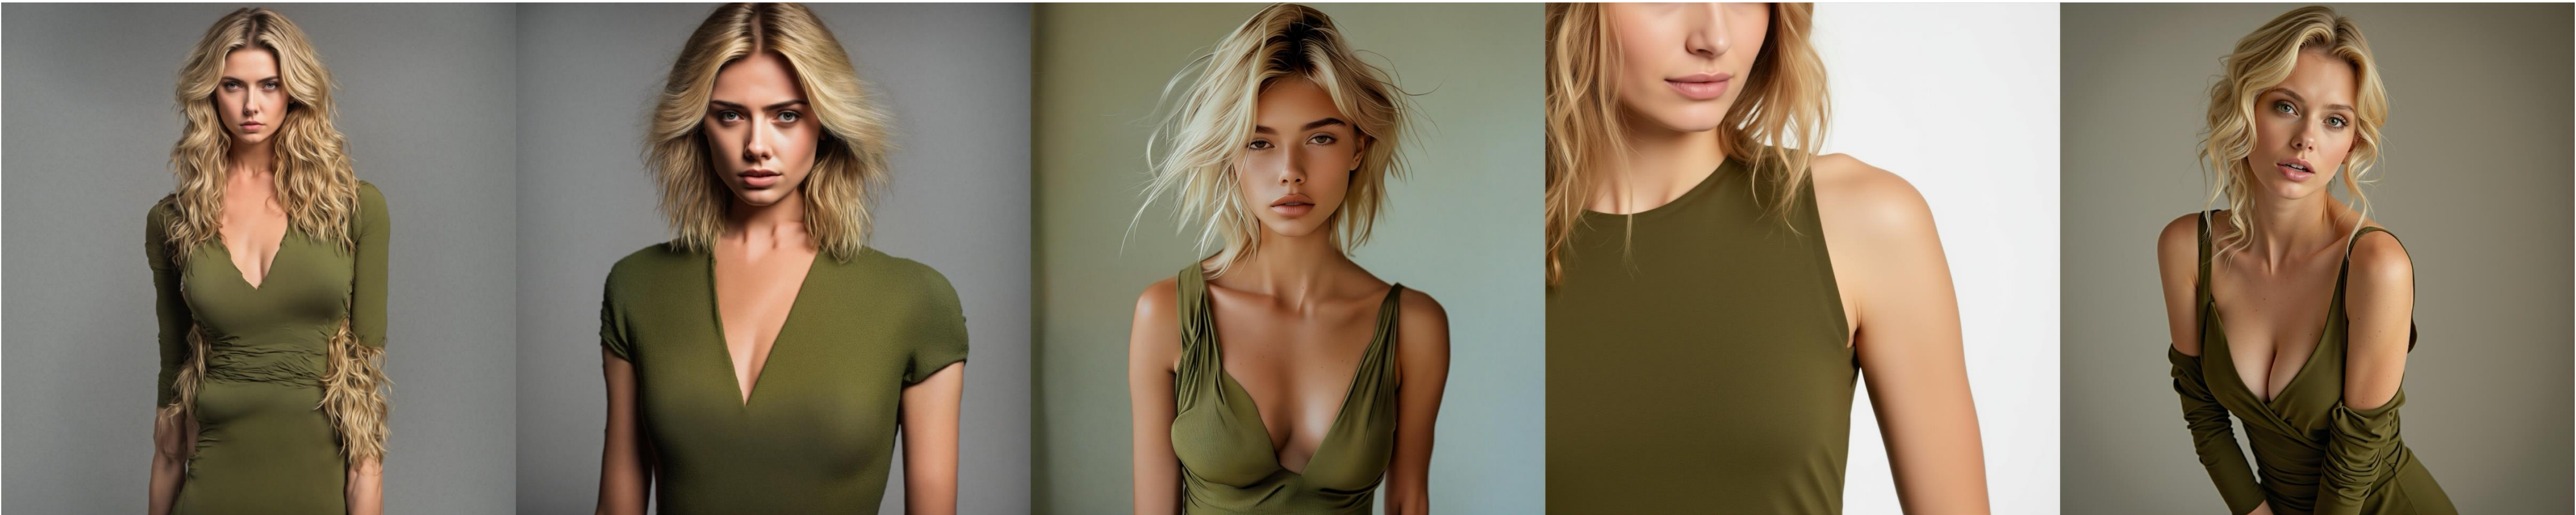

*An older man in a dark suit and fedora sits casually on a balcony, wearing sunglasses and holding a cigarette, with a serious expression against a muted background.*

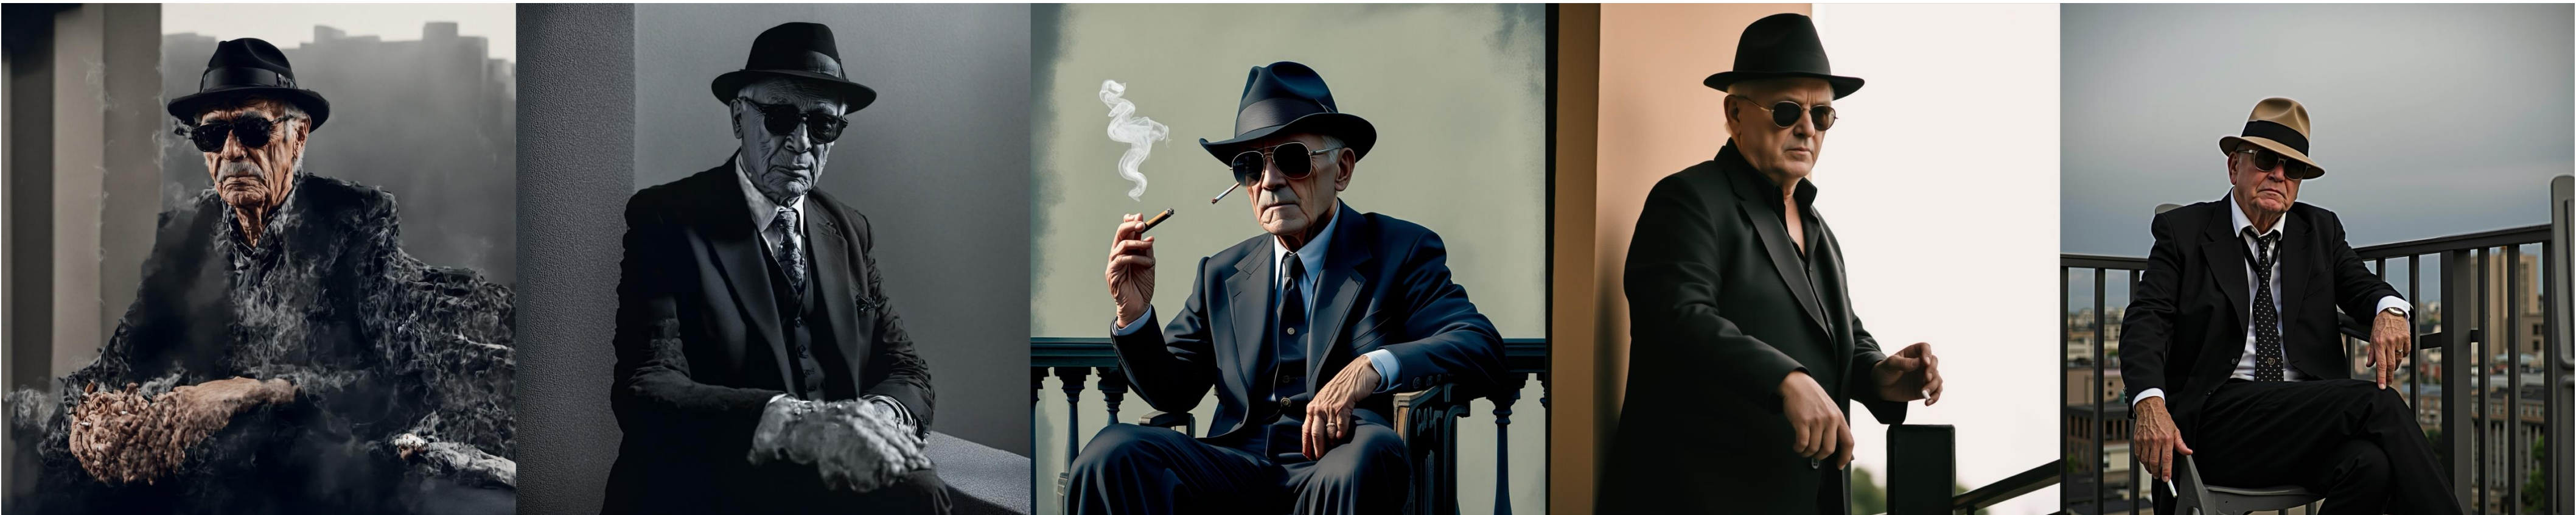

*A ballerina in a flowing yellow dress performs an elegant pose on one leg, showcasing her strength and grace against a backdrop of geometric wall art and soft natural light.*

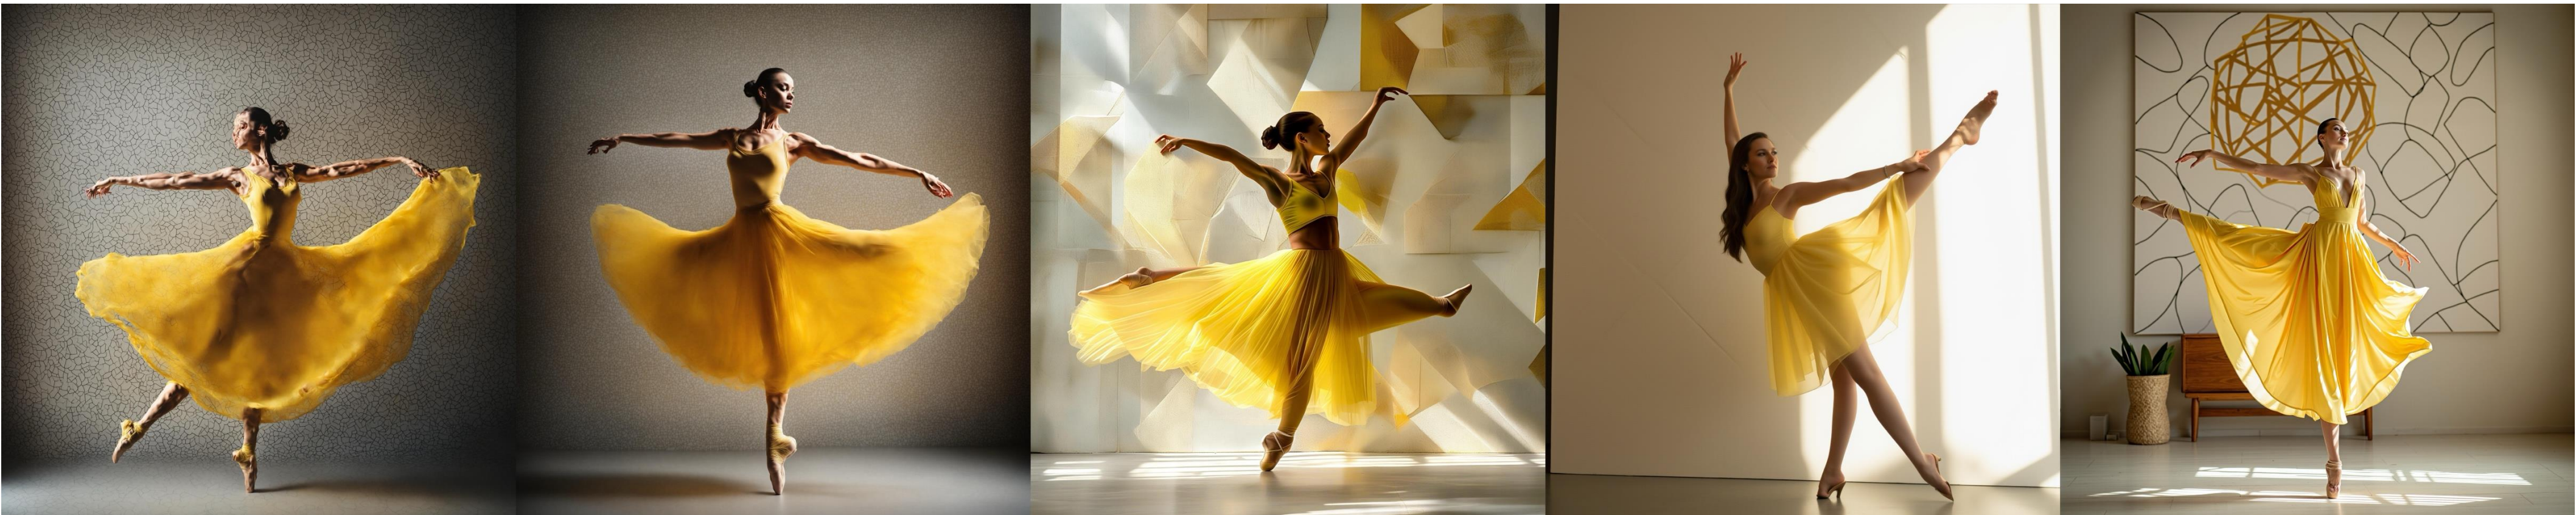

*A woman in a white dress with cape sleeves stands on a rooftop holding a black clutch, against a blurred city skyline and overcast sky.*

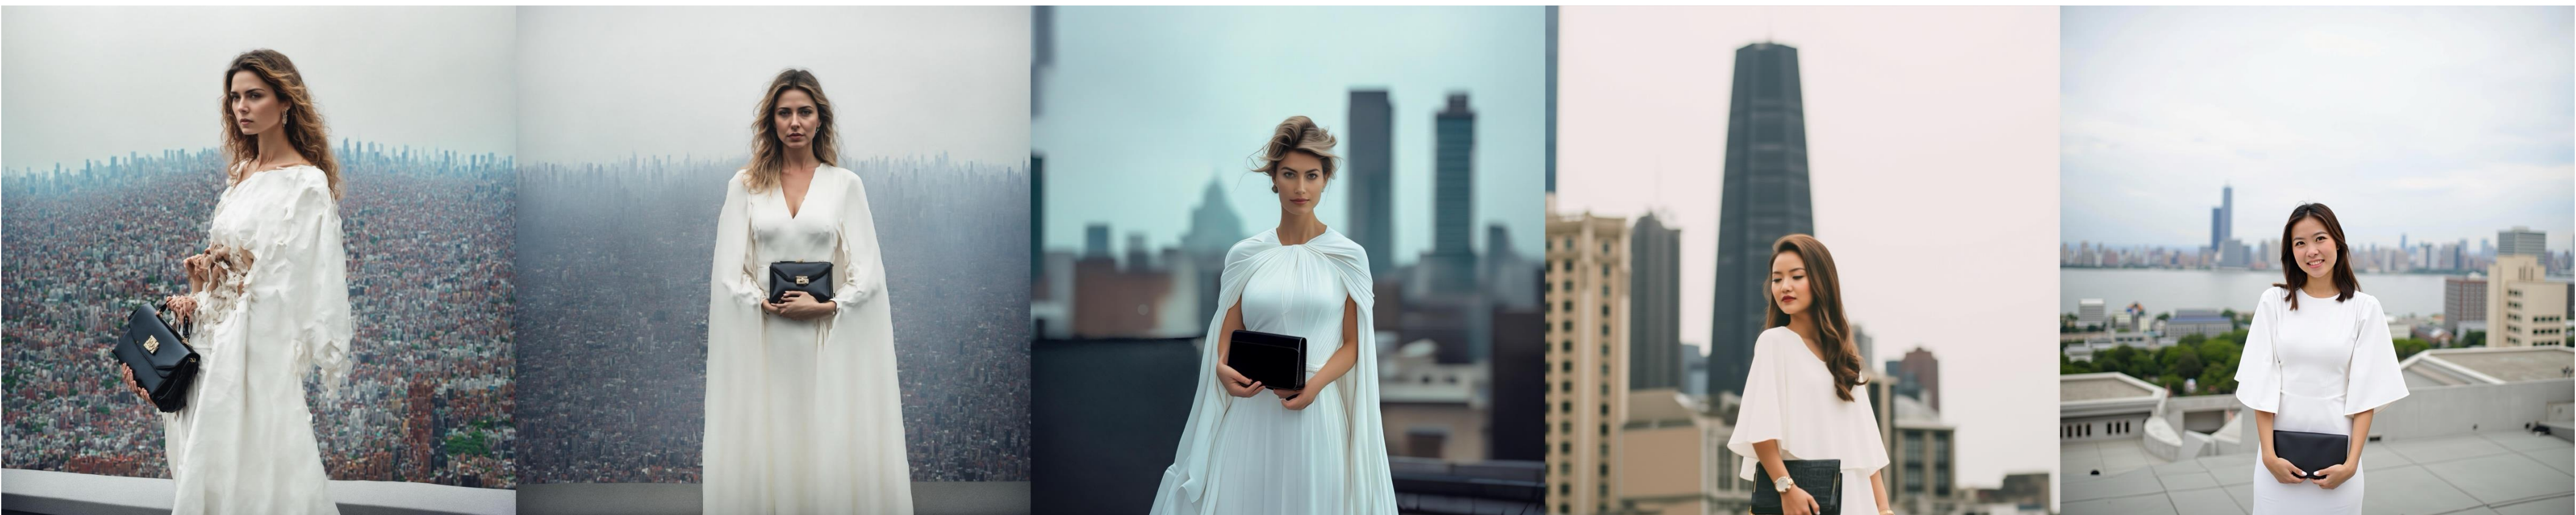

*A woman in a light blue dress stands at a balcony, holding onto the door frame, with a view of a serene coastal landscape featuring mountains and a peaceful shoreline.*

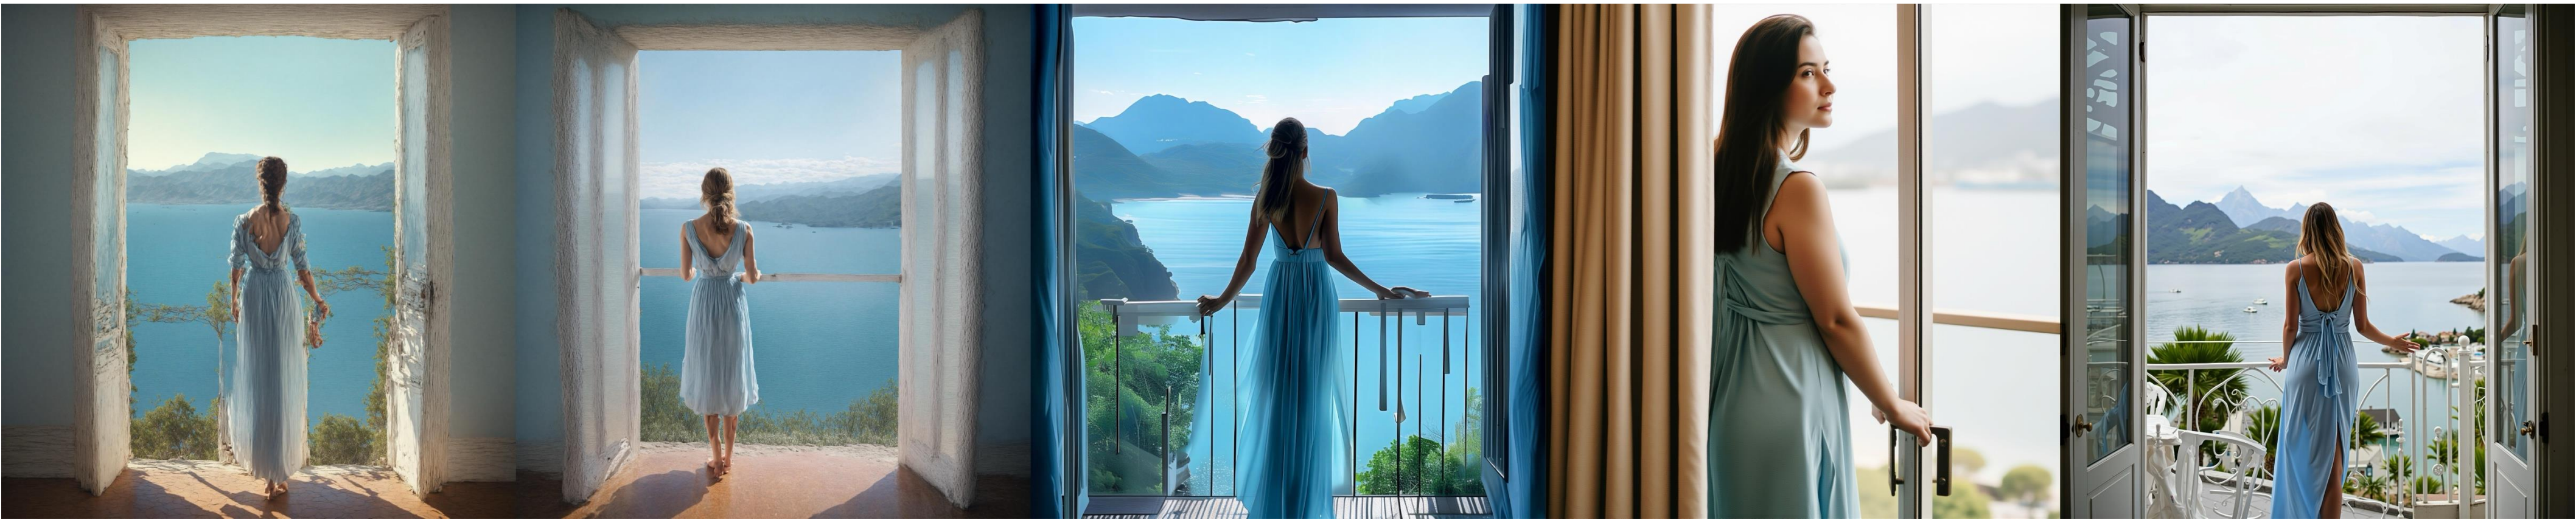

ScaleCrafter

FouriScale

SANA

Diffusion-4K

UltraFlux (Ours)

*A still life composition featuring two blue glass bottles next to a black bowl filled with several pears, set against a textured backdrop with warm tones.*

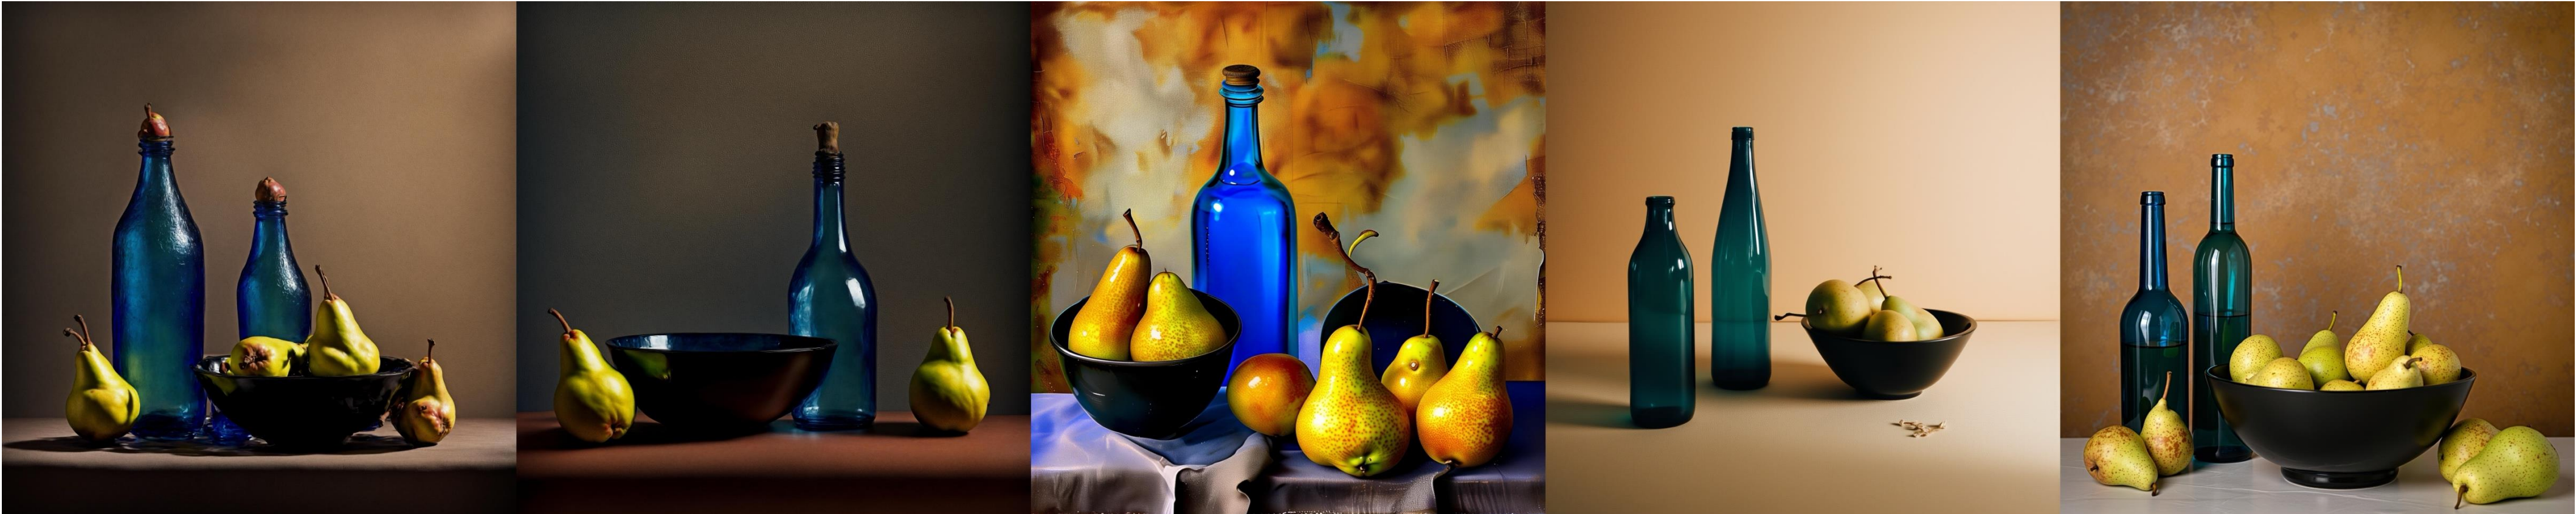

*A surfer rides a wave beneath the surface, showcasing skill and agility on a yellow board, with coral formations visible below.*

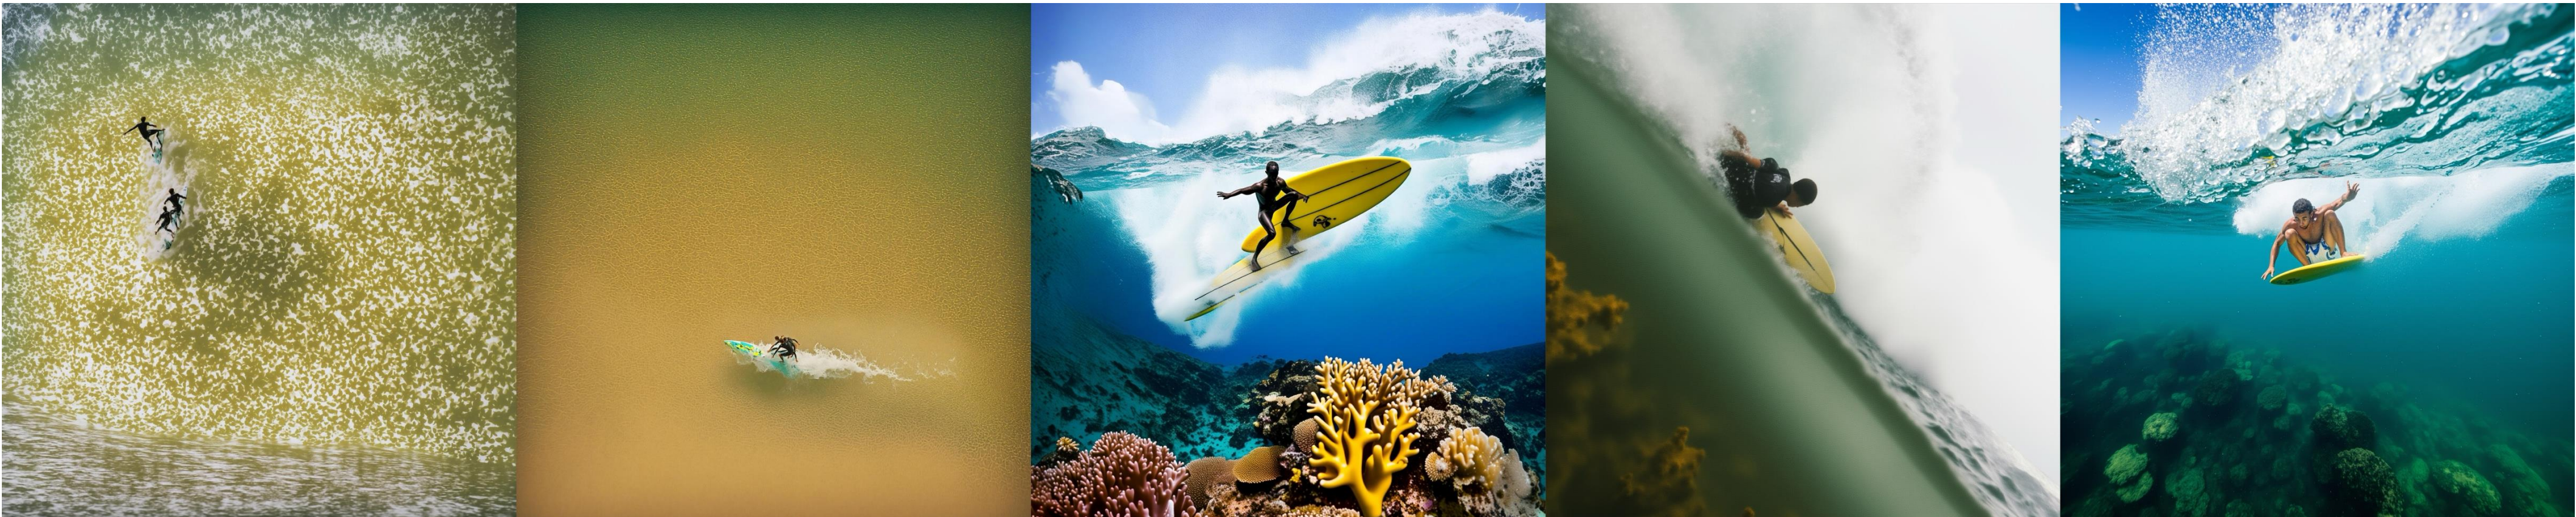

*A grand interior with soaring arches, intricate stonework, and vibrant stained glass windows, illuminated by ornate chandeliers and soft light, creating an atmosphere of reverence and awe.*

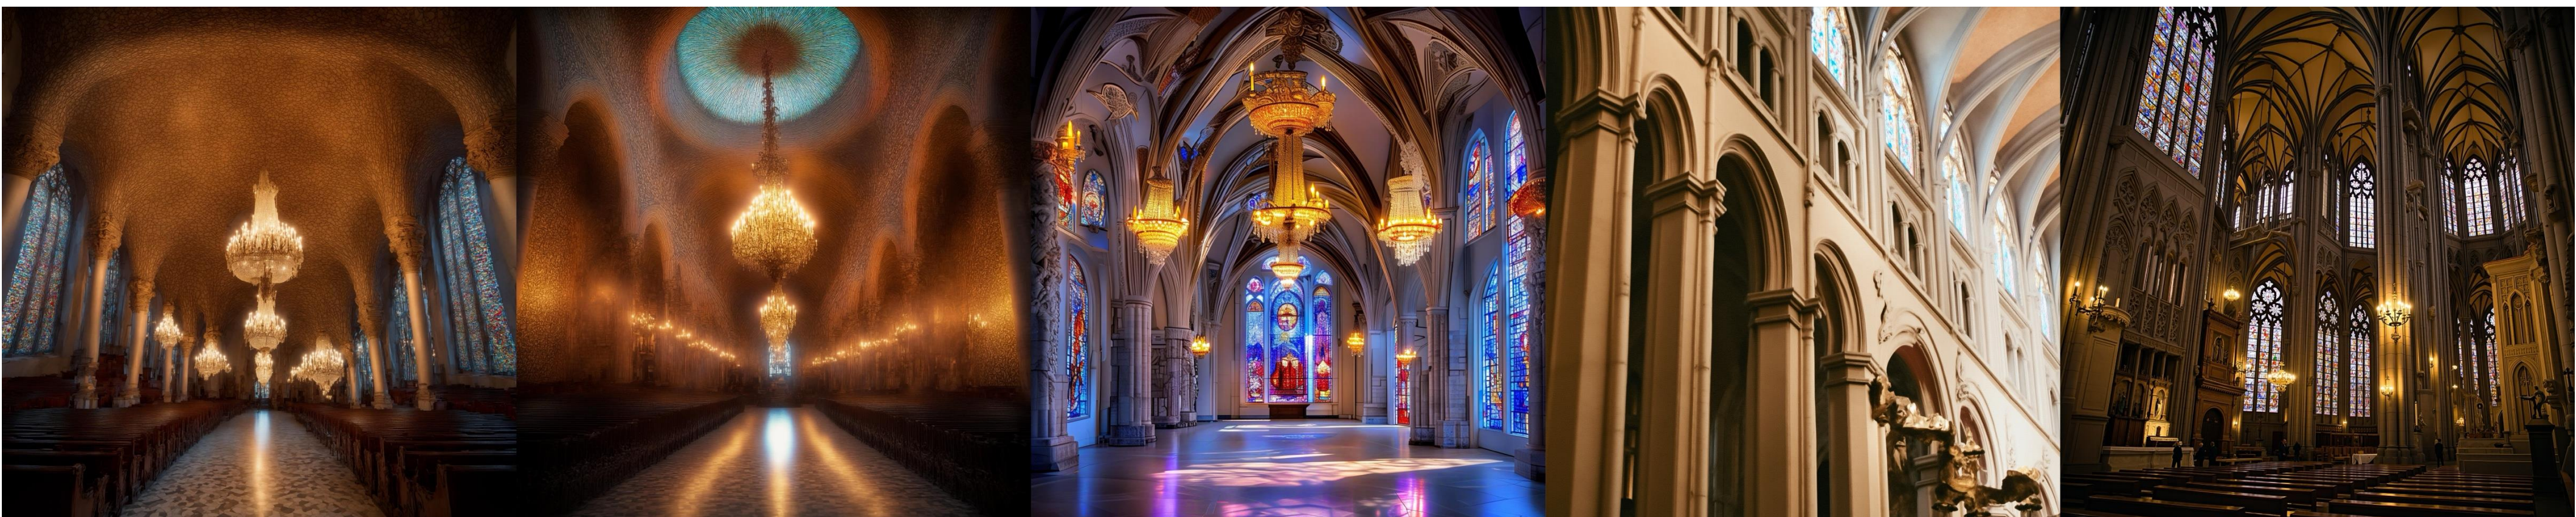

*A majestic waterfall cascades into a lush, green valley, surrounded by dense forest and towering mountains, with a mist hovering over the lower areas and a volcano rising in the background under a soft sky.*

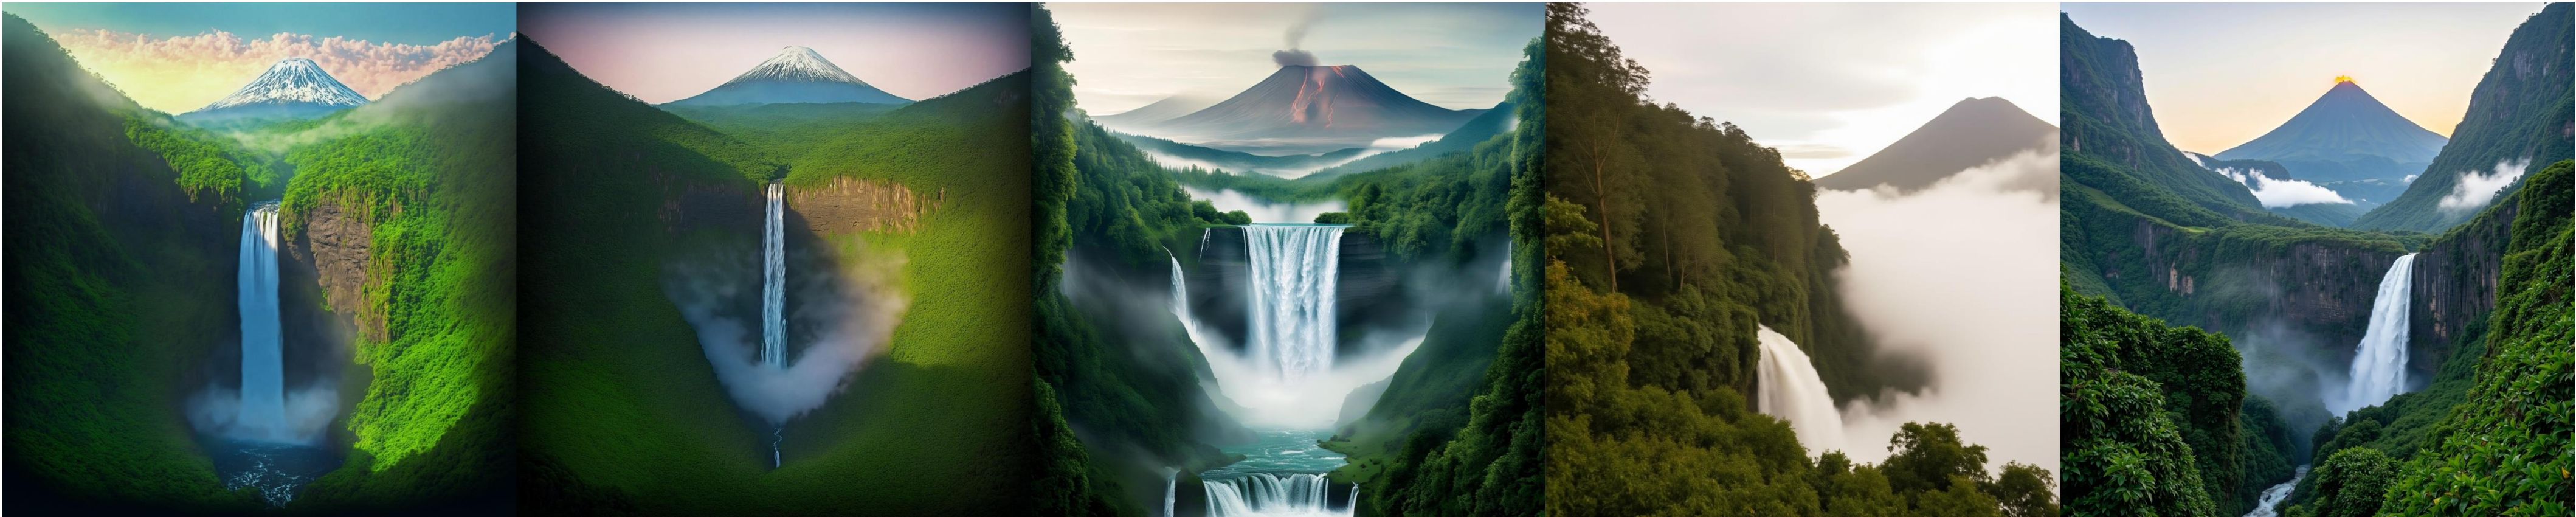

*Snow-capped mountains loom in the background, their peaks reflected in a calm lake surrounded by a rocky shore and green pine trees.*

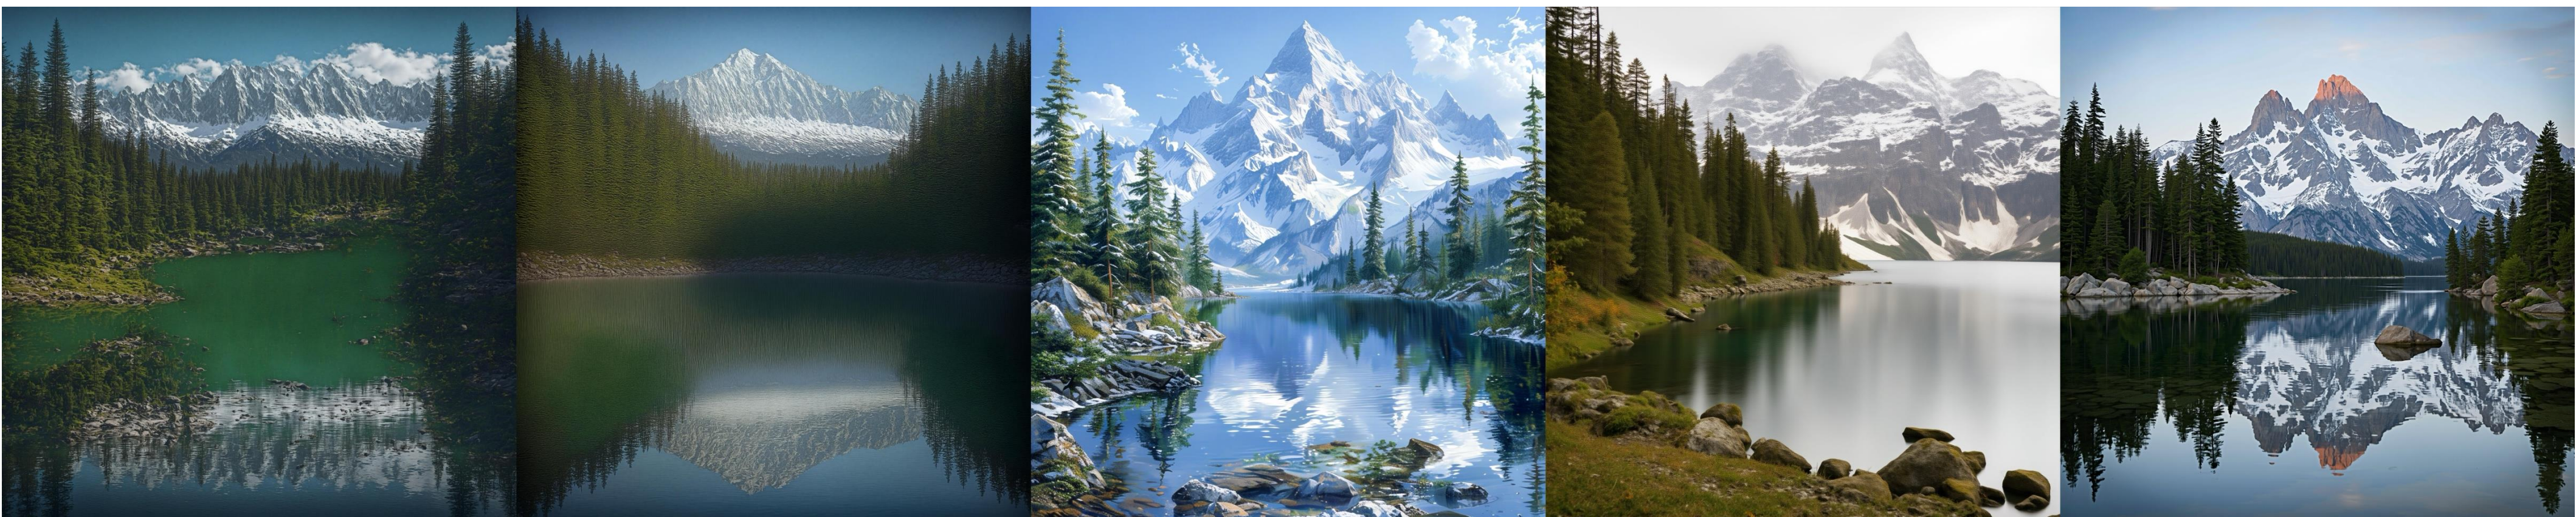

*A woman in a vintage, elegantly tailored gown with intricate embroidery gazes thoughtfully over a balcony, with a scenic river and historic buildings in the background.*

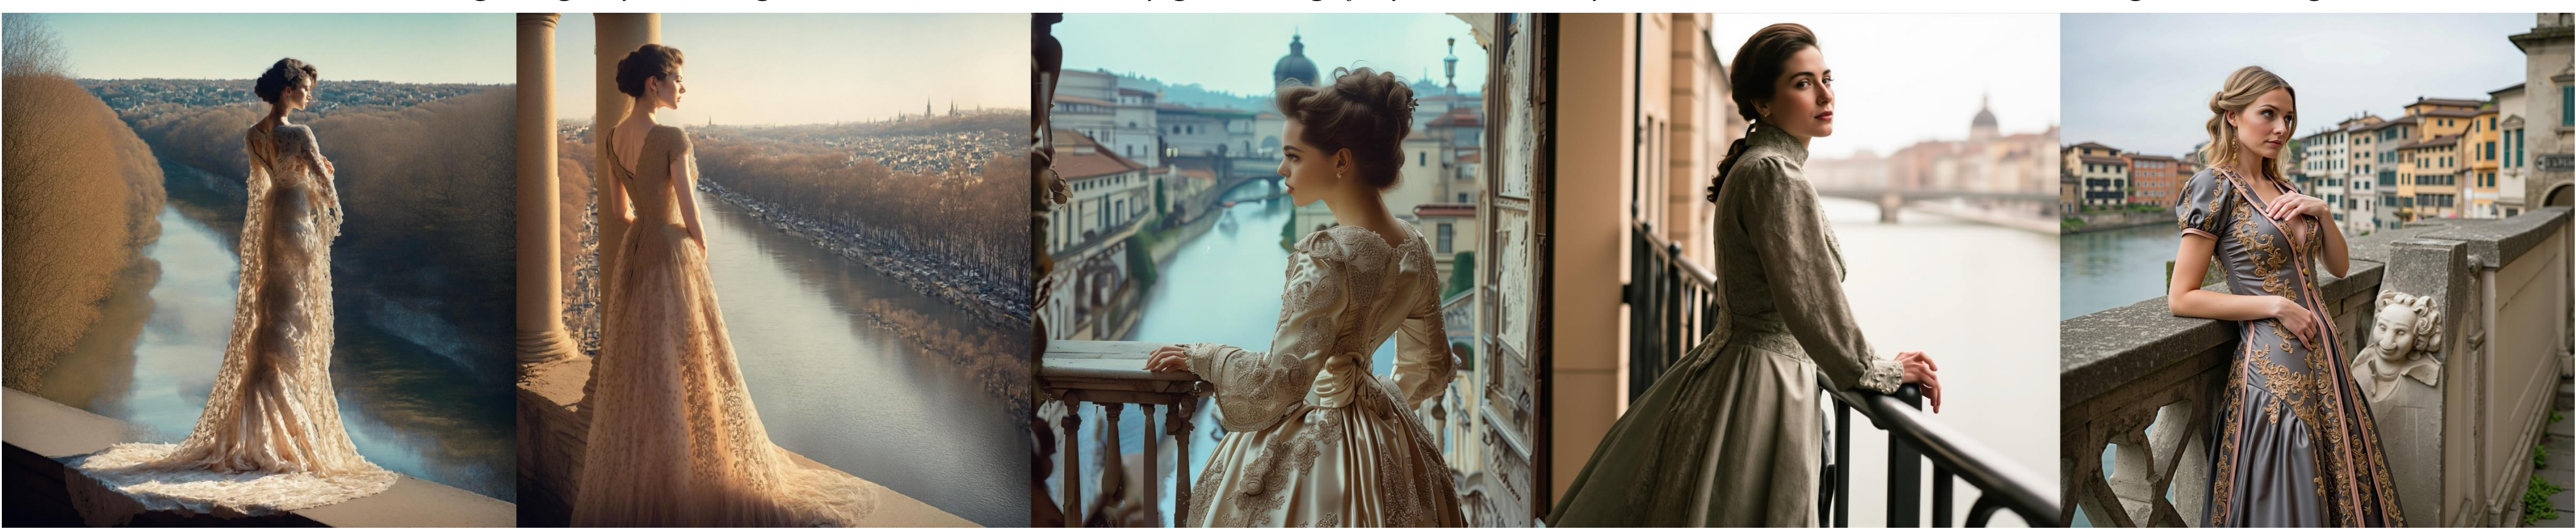

ScaleCrafter

FouriScale

SANA

Diffusion-4K

UltraFlux (Ours)

*A dramatic landscape featuring majestic, snow-capped mountains under a colorful rainbow, with dark, sandy terrain dotted with patches of grass.*

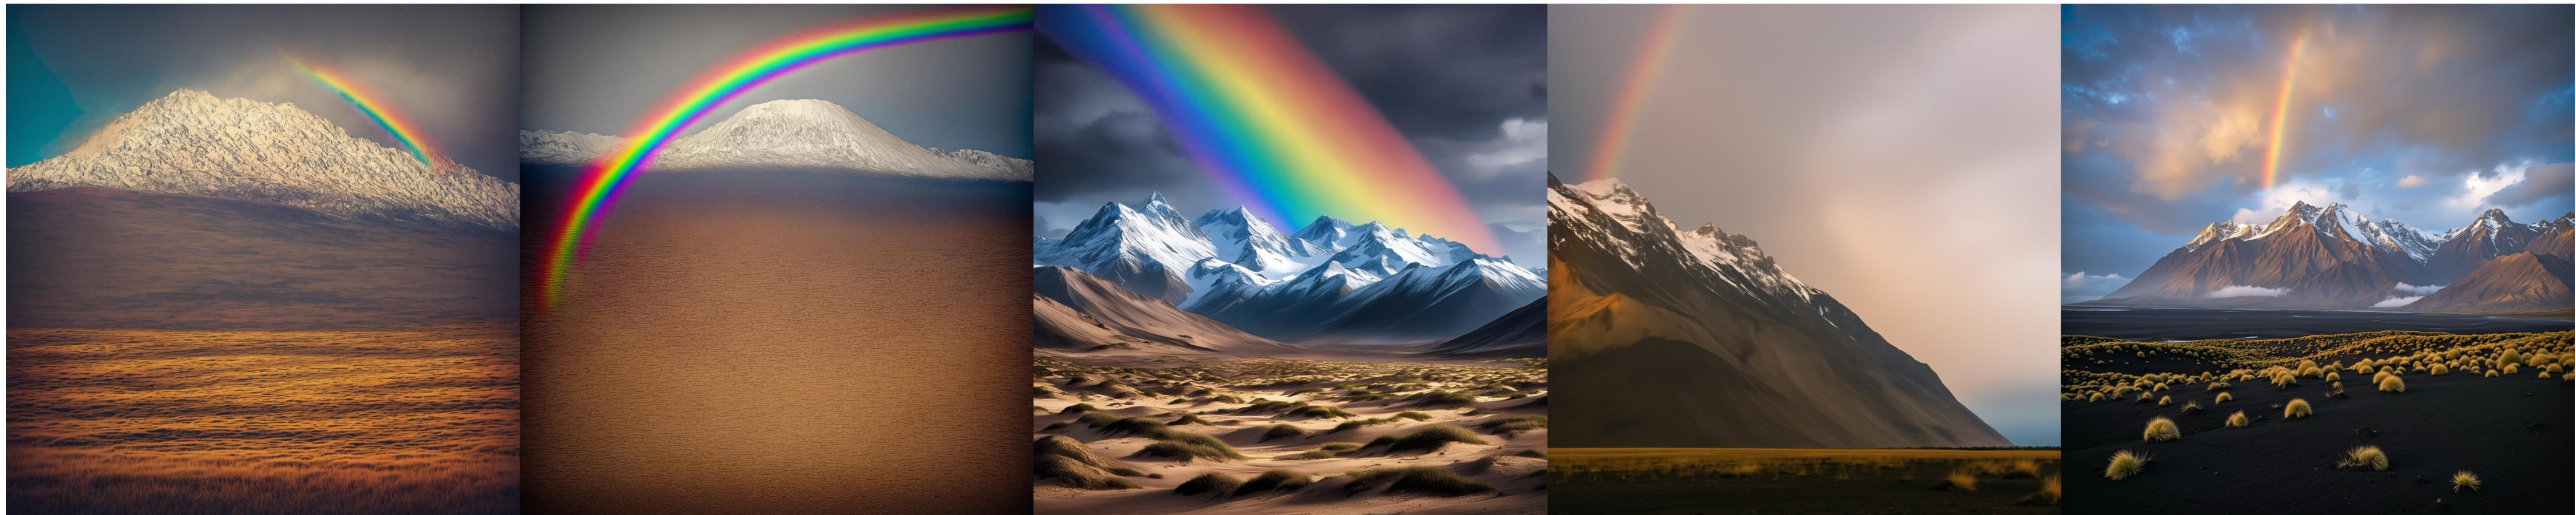

*A vibrant night sky filled with a milky way galaxy and swirling colors, reflected in a still, steaming geothermal pool surrounded by dark silhouettes of trees and misty atmosphere.*

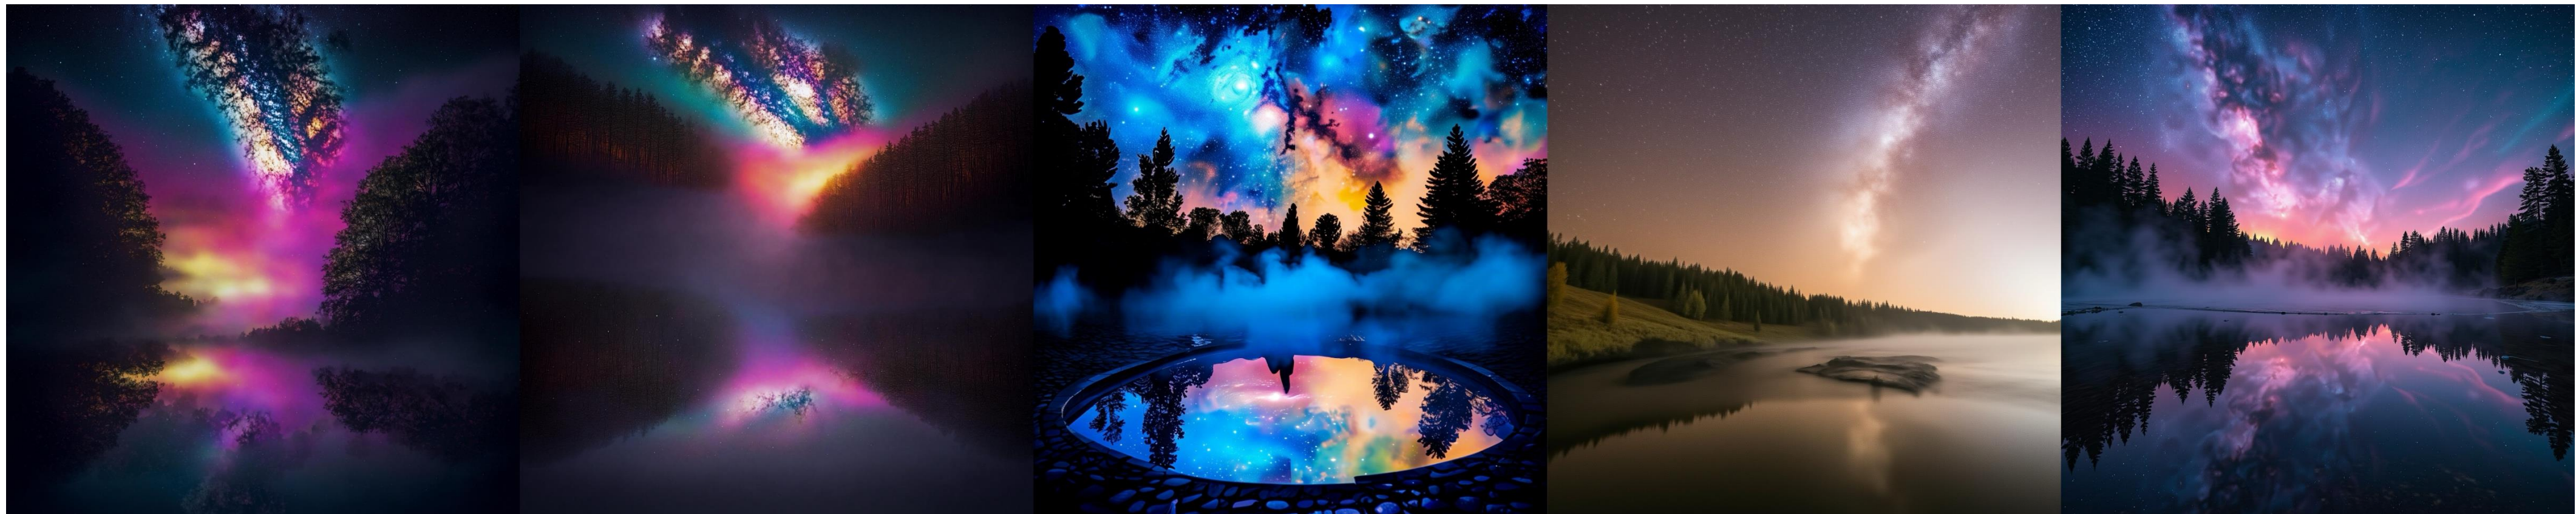

*A picturesque riverside scene featuring a medieval castle atop a hill, surrounded by vibrant autumn foliage, with colorful homes lining the waterfront and several boats docked along the river.*

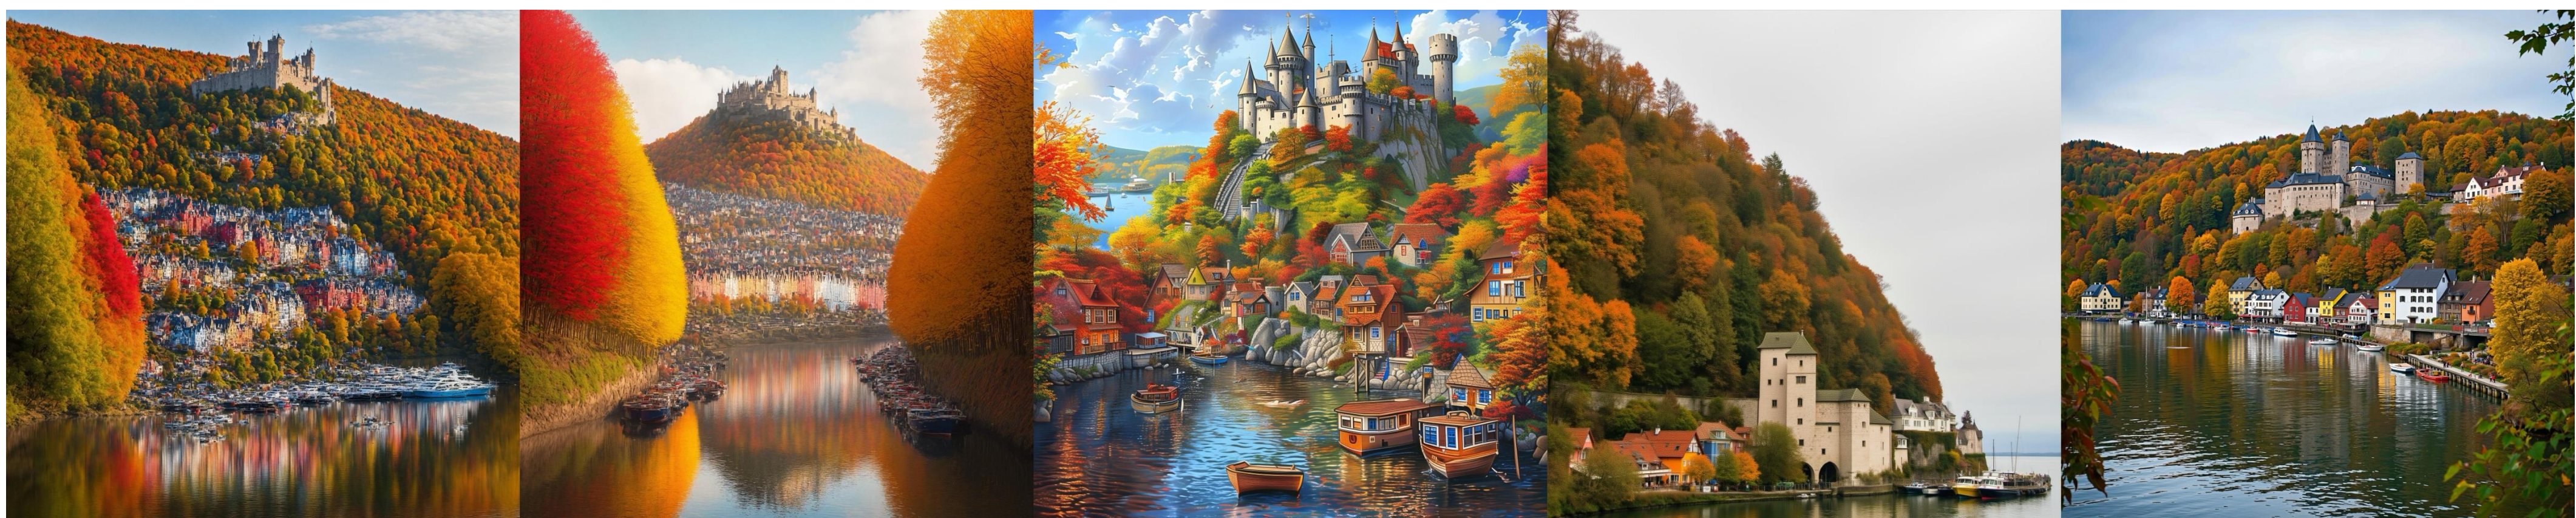

*Two individuals set up a tent on a grassy hillside, surrounded by mountains, with the sun rising in the background.*

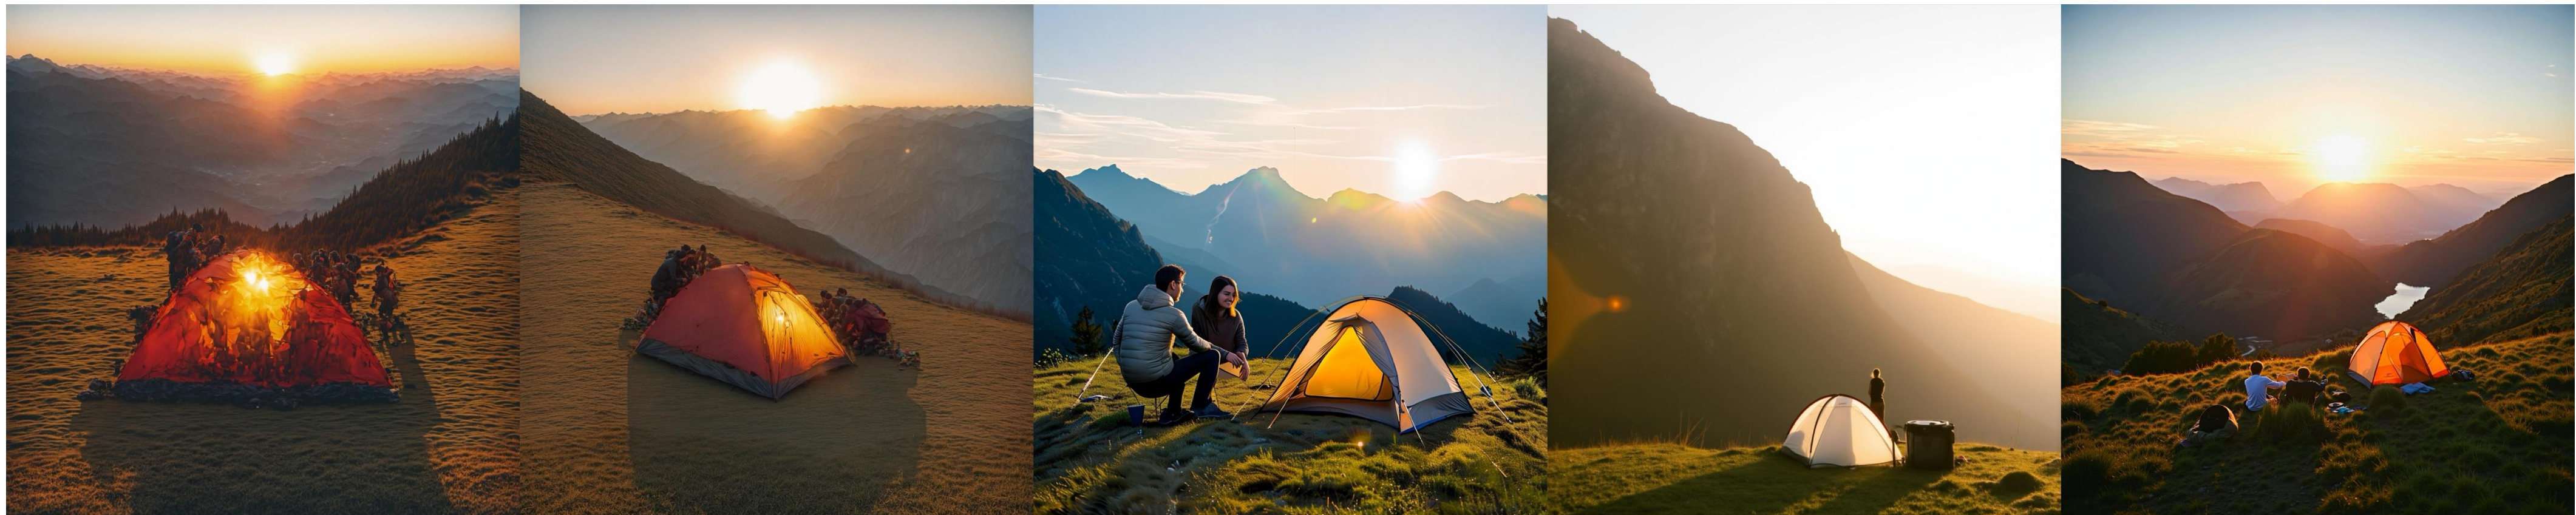

*A middle-aged man with long, gray hair and a short beard smiles gently, his warm, expressive eyes capturing attention against a dark background.*

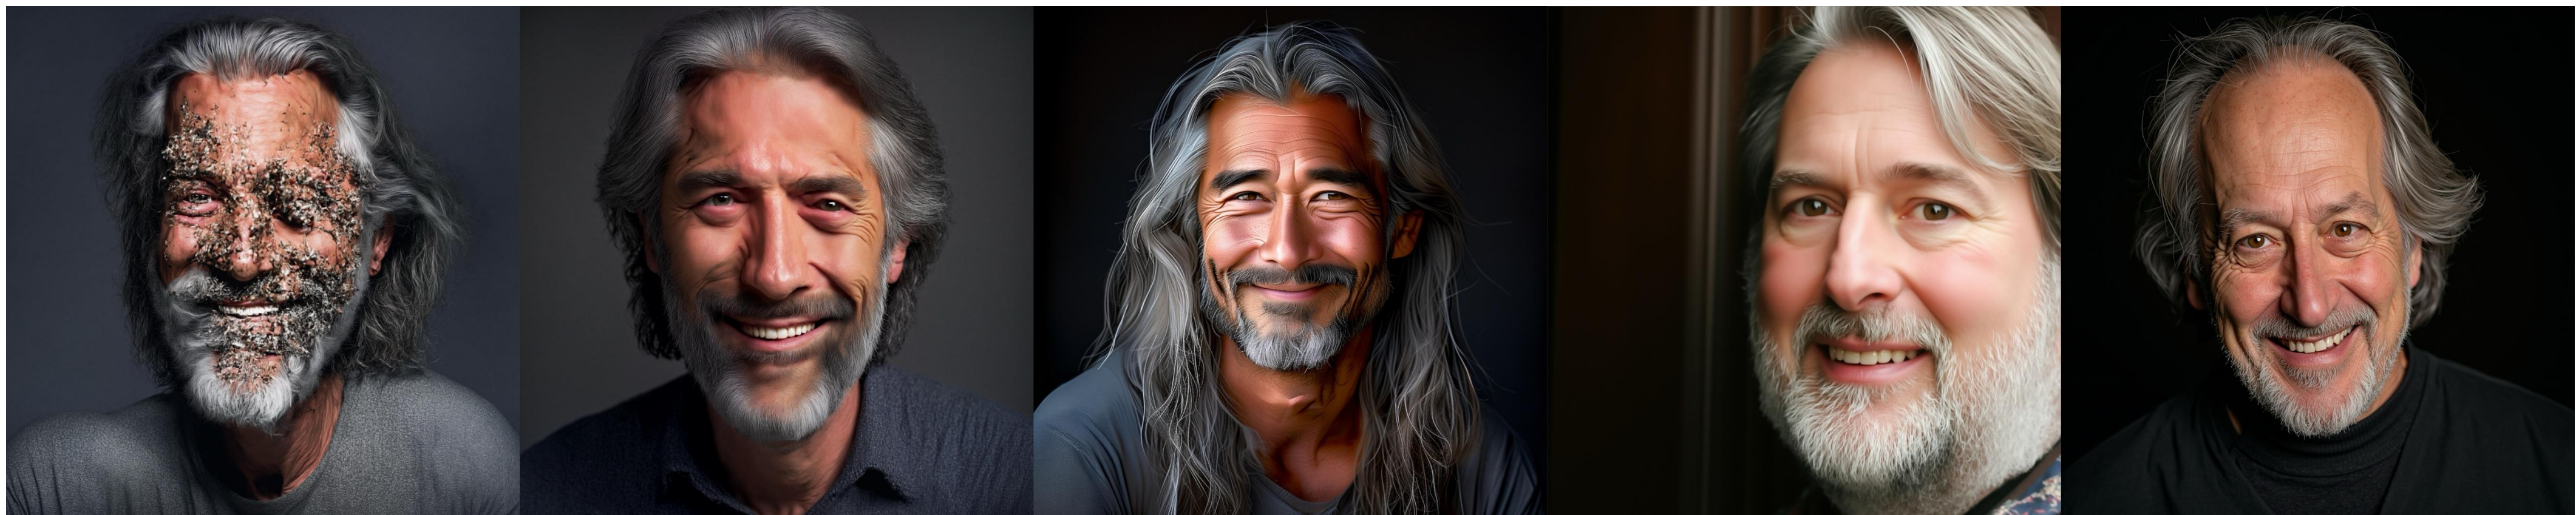

*A stone bridge with arched spans reflects golden light on the water, flanked by buildings and a leafy tree under a clear blue sky.*

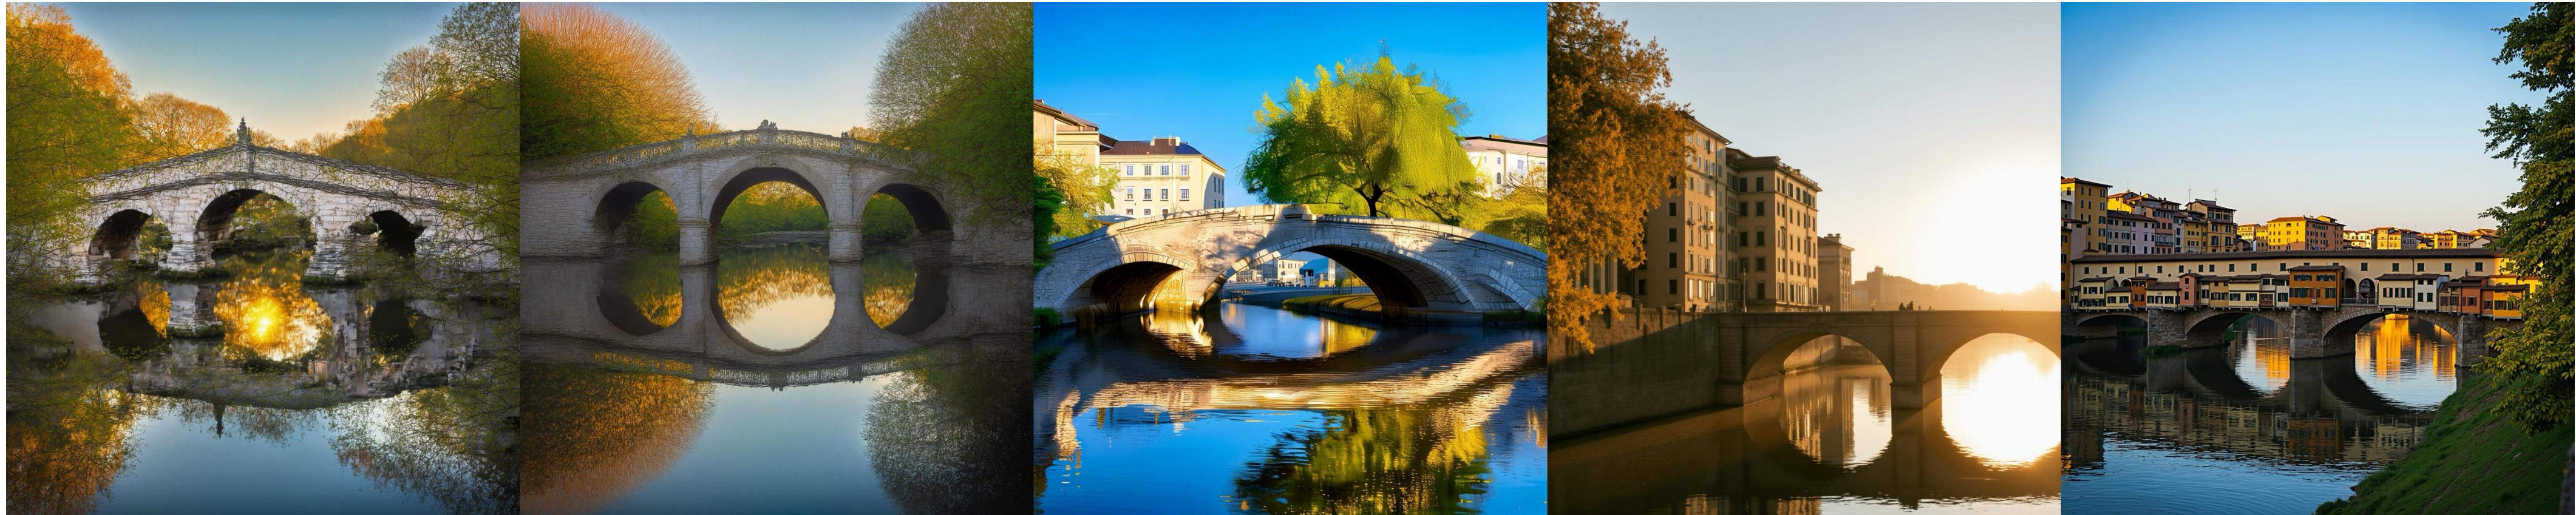

ScaleCrafter

FouriScale

SANA

Diffusion-4K

UltraFlux (Ours)
